# Supplementary material for: SalFBNet: Learning Pseudo-Saliency Distribution via Feedback Convolutional Networks
Source: arXiv:2112.03731 source file (2022-01-11)
Supplement: Supplementary file 1 [file FBNet_appendix.tex]

\newpage
\textbf{Appendix}

this is appendix.

\begin{table}[!ht]
\centering \caption{The $k$-folds standard deviation (STD) comparison of models with different filter sizes on SALICON \cite{jiang2015salicon} validation set.}
\resizebox{0.48\textwidth}{!}{
\begin{tabular}{  c | c  c  c  c  c  c  c }
\hline
\small \#Filter Size              & \small AUC-J $\uparrow$ &  \small AUC-B $\uparrow$   &  \small  sAUC $\uparrow$   & \small  CC $\uparrow$ & \small  NSS $\uparrow$ & \small  KLdiv $\downarrow$ & \small  SIM $\uparrow$  \\
\hline\hline
\small 8 & 0.0010     & 0.0020  & 0.0007 & 0.0026 & 0.0042    & 0.0601  & 0.0019 \\
\small 16 & 0.0009     & 0.0014  & 0.0014 & 0.0048 & 0.0177    & 0.0710  & 0.0069 \\
\small 32 & 0.0001     & 0.0009  & 0.0009 & 0.0002 & 0.0026    & 0.0395  & 0.0033 \\
\small 64 & 0.0010     & 0.0007  & 0.0005 & 0.0053 & 0.0150    & 0.0368  & 0.0080 \\
\small 96 & 0.0005     & 0.0033  & 0.0015 & 0.0048 & 0.0183    & 0.0519  & 0.0172 \\
\small 128 & 0.0004     & 0.0015  & 0.0012 & 0.0021 & 0.0070    & 0.0185  & 0.0048 \\
\small 160 & 0.0010     & 0.0031  & 0.0010 & 0.0023 & 0.0059    & 0.0261  & 0.0043 \\
\small 196 & 0.0017     & 0.0028  & 0.0030 & 0.0078 & 0.0132    & 0.0516  & 0.0028 \\
\hline
\end{tabular}
}
\label{tab:filtersize_comp_std}
\end{table}

\begin{table*}[ht!]
\centering \caption{Quantitative performance of different methods on pseudo-saliency dataset.}
\resizebox{0.94\textwidth}{!}{
\begin{tabular}{  c | c  c  c  c  c | c  c  c  c  c | c  c  c  c  c }
\hline
\small & \multicolumn{15}{c}{\textbf{SALICON \cite{jiang2015salicon} training Set}}   \\
\hline
\small Metric &  \multicolumn{5}{c|}{CC} &  \multicolumn{5}{c|}{KLdiv} &  \multicolumn{5}{c}{SIM}   \\
\hline
\small Model              & \small MSINet  \cite{kroner2020contextual} &  \small DeepGaze  \cite{linardos2021deepgaze}   &  \small EMLNet  \cite{jia2020eml}   & \small  CASNet   \cite{fan2018emotional} & \small  UNISAL \cite{droste2020unified} & \small MSINet  \cite{kroner2020contextual} &  \small DeepGaze  \cite{linardos2021deepgaze}   &  \small EMLNet  \cite{jia2020eml}   & \small  CASNet   \cite{fan2018emotional} & \small  UNISAL \cite{droste2020unified} & \small MSINet  \cite{kroner2020contextual} &  \small DeepGaze  \cite{linardos2021deepgaze}   &  \small EMLNet  \cite{jia2020eml}   & \small  CASNet   \cite{fan2018emotional} & \small  UNISAL \cite{droste2020unified} \\
\hline\hline
\small MSINet  \cite{kroner2020contextual} & 1.0000     & 0.8400  & 0.9419 & 0.9180 & 0.8292    & 0.0000  & 0.4235 & 0.5756     & 0.1795  & 0.5147 & 1.0000 & 0.7410    & 0.8440  & 0.8058 & 0.7422 \\
\small DeepGaze  \cite{linardos2021deepgaze}               & 0.8400     & 1.0000  & 0.8140 & 0.8245 & 0.7076     & 0.3982  & 0.0000 & 1.0503 & 0.2780     & 0.8089  & 0.7410 & 1.0000 & 0.7188 & 0.7230 & 0.7459   \\
\small EMLNet  \cite{jia2020eml} & 0.9419     & 0.8140  & 1.0000 & 0.8849 & 0.8431     & 0.1082  & 0.3642 & 0.0000 & 0.2606     & 0.4106  & 0.8440 & 0.7188 & 1.0000 & 0.7525 & 0.7268  \\
\small CASNet   \cite{fan2018emotional} & 0.9180     & 0.8245  & 0.8849 & 1.0000 & 0.7964     & 0.7473  & 0.8733 & 1.8980 & 0.0000     & 1.1199  & 0.8058 & 0.7230 & 0.7525 & 1.0000 & 0.7190  \\
\small UNISAL \cite{droste2020unified} & 0.8292     & 0.7076  & 0.8431 & 0.7964 & 1.0000     & 0.7229  & 1.1197 & 1.7512 & 0.4157     & 0.0000  & 0.7422 & 0.6459 & 0.7268 & 0.7190 & 1.0000  \\
\hline
\small & \multicolumn{15}{c}{\textbf{SALICON \cite{jiang2015salicon} validation Set}}   \\
\hline
\small Metric &  \multicolumn{5}{c|}{CC} &  \multicolumn{5}{c|}{KLdiv} &  \multicolumn{5}{c}{SIM}   \\
\hline
\small Model              & \small MSINet  \cite{kroner2020contextual} &  \small DeepGaze  \cite{linardos2021deepgaze}   &  \small EMLNet  \cite{jia2020eml}   & \small  CASNet   \cite{fan2018emotional} & \small  UNISAL \cite{droste2020unified} & \small MSINet  \cite{kroner2020contextual} &  \small DeepGaze  \cite{linardos2021deepgaze}   &  \small EMLNet  \cite{jia2020eml}   & \small  CASNet   \cite{fan2018emotional} & \small  UNISAL \cite{droste2020unified} & \small MSINet  \cite{kroner2020contextual} &  \small DeepGaze  \cite{linardos2021deepgaze}   &  \small EMLNet  \cite{jia2020eml}   & \small  CASNet   \cite{fan2018emotional} & \small  UNISAL \cite{droste2020unified} \\
\hline\hline
\small MSINet  \cite{kroner2020contextual} & 1.0000     & 0.8414  & 0.9330 & 0.9051 & 0.8261    & 0.0000  & 0.4331 & 0.6109     & 0.1866  & 0.5503 & 1.0000 & 0.7438    & 0.8311  & 0.7970 & 0.7428 \\
\small DeepGaze  \cite{linardos2021deepgaze}               & 0.8414     & 1.0000  & 0.8272 & 0.8132 & 0.7079     & 0.3679  & 0.0000 & 0.9051 & 0.2962     & 0.8348  & 0.7438 & 1.0000 & 0.7303 & 0.7139 & 0.6466   \\
\small EMLNet  \cite{jia2020eml} & 0.9330     & 0.8272  & 1.0000 & 0.8754 & 0.8528     & 0.1279  & 0.3420 & 0.0000 & 0.2655     & 0.4030  & 0.8311 & 0.7303 & 1.0000 & 0.7464 & 0.7381  \\
\small CASNet   \cite{fan2018emotional} & 0.9051     & 0.8132  & 0.8754 & 1.0000 & 0.7862     & 0.7595  & 0.9620 & 1.8652 & 0.0000     & 1.2567  & 0.7970 & 0.7139 & 0.7464 & 1.0000 & 0.7107\\
\small UNISAL \cite{droste2020unified} & 0.8261     & 0.7079  & 0.8528 & 0.7862 & 1.0000     & 0.6434  & 1.1005 & 1.4857 & 0.4227     & 0.0000  & 0.7428 & 0.6466 & 0.7381 & 0.7107 & 1.0000  \\
\hline
\end{tabular}
}
\label{tab:pseoudo_comp_distribution}
\end{table*}

\begin{table}[!ht]
\centering \caption{The $k$-folds performance of different filter sizes on SALICON \cite{jiang2015salicon} validation dataset.}
\resizebox{0.48\textwidth}{!}{
\begin{tabular}{  c | c  c  c  c  c  c  c }
\hline
\small ~ &  \multicolumn{7}{c}{\textbf{1st fold}}   \\
\hline
\small \#Filter Size              & \small AUC-J $\uparrow$ &  \small AUC-B $\uparrow$   &  \small  sAUC $\uparrow$   & \small  CC $\uparrow$ & \small  NSS $\uparrow$ & \small  KLdiv $\downarrow$ & \small  SIM $\uparrow$  \\
\hline\hline
\small 8 & 0.8357     & 0.8206  & 0.6886 & 0.7449 & 1.5314    & 0.7027  & 0.6576 \\
\small 16 & 0.8431     & 0.8308  & 0.6959 & 0.7697 & 1.5800    & 0.4627  & 0.6664 \\
\small 32 & 0.8485     & 0.8322  & 0.7060 & 0.7954 & 1.6553    & 0.4620  & 0.6877 \\
\small 64 & 0.8505     & 0.8351  & 0.7105 & 0.8032 & 1.6777    & 0.4588  & 0.6913 \\
\small 96 & 0.8495     & 0.8381  & 0.7080 & 0.7985 & 1.6592    & 0.4208  & 0.6642 \\
\small 128 & 0.8511     & 0.8355  & 0.7129 & 0.8058 & 1.6870    & 0.3952  & 0.6903 \\
\small 160 & 0.8505     & 0.8366  & 0.7138 & 0.8022 & 1.6797    & 0.3821  & 0.6811 \\
\small 196 & 0.8484     & 0.8331  & 0.7095 & 0.7937 & 1.6630    & 0.4763  & 0.6832 \\
\hline
\small ~ &  \multicolumn{7}{c}{\textbf{2nd fold}}   \\
\hline
\small 8 & 0.8377     & 0.8246  & 0.6885 & 0.7499 & 1.5386    & 0.5835  & 0.6565 \\
\small 16 & 0.8445     & 0.8316  & 0.6972 & 0.7759 & 1.5981    & 0.4466  & 0.6674 \\
\small 32 & 0.8486     & 0.8341  & 0.7075 & 0.7954 & 1.6576    & 0.3920  & 0.6813 \\
\small 64 & 0.8485     & 0.8360  & 0.7094 & 0.7933 & 1.6491    & 0.4480  & 0.6772 \\
\small 96 & 0.8504     & 0.8316  & 0.7102 & 0.8076 & 1.6954    & 0.4838  & 0.6985 \\
\small 128 & 0.8503     & 0.8352  & 0.7115 & 0.8107 & 1.6738    & 0.4214  & 0.6896 \\
\small 160 & 0.8505     & 0.8383  & 0.7120 & 0.8005 & 1.6680    & 0.3966  & 0.6773 \\
\small 196 & 0.8508     & 0.8367  & 0.7149 & 0.8054 & 1.6841    & 0.3860  & 0.6847 \\
\hline
\small ~ &  \multicolumn{7}{c}{\textbf{3rd fold}}   \\
\hline
\small 8 & 0.8362     & 0.8226  & 0.6874 & 0.7467 & 1.5312    & 0.6562  & 0.6538 \\
\small 16 & 0.8446     & 0.8289  & 0.6986 & 0.7792 & 1.6154    & 0.5768  & 0.6789 \\
\small 32 & 0.8484     & 0.8332  & 0.7057 & 0.7951 & 1.6525    & 0.4586  & 0.6862 \\
\small 64 & 0.8502     & 0.8365  & 0.7100 & 0.8013 & 1.6715    & 0.3903  & 0.6776 \\
\small 96 & 0.8505     & 0.8354  & 0.7072 & 0.8059 & 1.6815    & 0.3810  & 0.6833 \\
\small 128 & 0.8508     & 0.8379  & 0.7105 & 0.8043 & 1.6763    & 0.3858  & 0.6817 \\
\small 160 & 0.8488     & 0.8323  & 0.7135 & 0.7977 & 1.6750    & 0.4328  & 0.6860 \\
\small 196 & 0.8517     & 0.8386  & 0.7099 & 0.8084 & 1.6872    & 0.3878  & 0.6793 \\
\hline
\end{tabular}
}
\label{tab:filter_size_comp_k}
\end{table}
